# Supplementary material for: Unraveling the water degradation mechanism of CH$_3$NH$_3$PbI$_3$
Source: arXiv:1905.12494 source file (2019-08-27)
Supplement: Supplementary file 1 [file Supporting_information.pdf]

# Supporting Information

## Unraveling the Water Degradation Mechanism of $CH_3NH_3PbI_3$

Chao Zheng* and Oleg Rubel *

*Department of Materials Science and Engineering, McMaster University,*

*1280 Main Street West, Hamilton, Ontario L8S 4L8, Canada*

The free energy surface of $MA^+$ dissolution in water is plotted in FIG. S1. This free energy surface is only for initial basin. It is obtained via ~4.7 ps metadynamics with a Gaussian height of 0.026 and a Gaussian weight of 0.014 and a continuous ~4.6 ps metadynamic calculation with a Gaussian height of 0.052 and a Gaussian weight of 0.018. We found the case of $MA^+$ calculation took much longer time staying at the initial basin. Due to the capability of our facility and limited time, we stopped for exploring the sequent free energy surface of $MA^+$ dissolution in water.

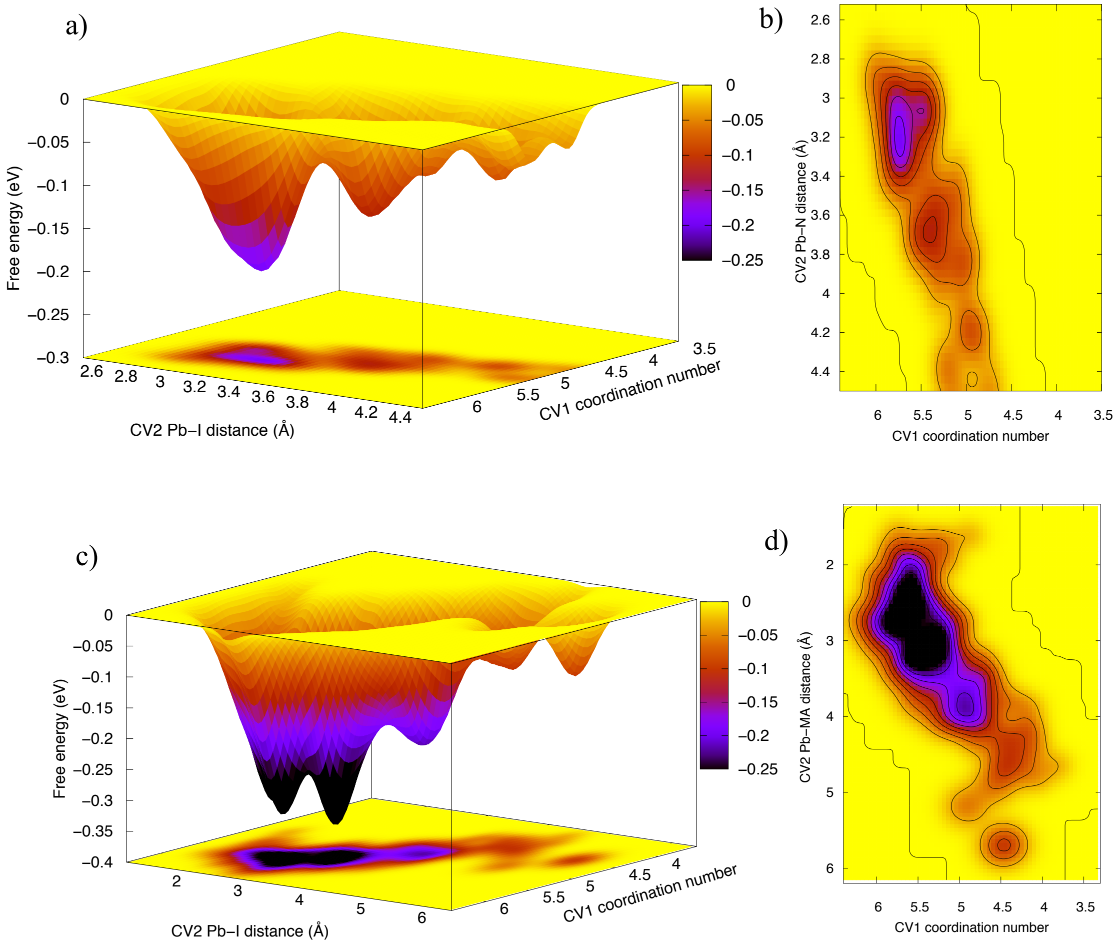


FIG. S1. (a) Free energy surface of initial basin of $I^-$ dissolution in water. (b) Contour of the free energy surface of $I^-$ dissolution in water. (c) Free energy surface of initial basin of $MA^+$ dissolution in water. (d) Contour of the free energy surface of $MA^+$ dissolution in water.

Comparing FIG. S1(a) and FIG. S1(c), we found the initial basin of $MA^+$ dissolution in water is deeper (~0.15 eV lower) than the value of $I^-$ dissolution in water. And from FIG. S1(b) and FIG. S1(d), we found the initial basin of $MA^+$ dissolution in water is wider than the case of $I^-$ dissolution in water. Hence, it explains the slow exploring rate and the inferiority of $MA^+$ dissolution in water for metadynamics.
